# Supplementary material for: Coherent THz Spin Dynamics in Antiferromagnets Beyond the Approximation of the N\'eel vector
Source: arXiv:2303.06996 ancillary file (2023-12-28)
Supplement: Supplementary file 1 [file RbMnF3_2magnon_SM.pdf]

# Supplemental Material to: Coherent THz Spin Dynamics in Antiferromagnets Beyond the Approximation of the Néel vector

F. Formisano [1], T. T. Gareev [1], D. I. Khusyainov [1], A. E. Fedianin [2], R. M. Dubrovin [2], P. P. Syrnikov [2], D. Afanasiev [1], R. V. Pisarev [2], A. M. Kalashnikova [2], J. H. Mentink [1], and A. V. Kimel [1, *]

[1] *Institute for Molecules and Materials, Radboud University, 6525 AJ Nijmegen, The Netherlands*
[2] *Ioffe Institute, Russian Academy of Sciences, 194021 St. Petersburg, Russia*

(Dated: December 18, 2023)

In this supplementary information we present a more detailed derivation of the equation of motion for spin correlations, equation for $\varepsilon^{xx} - \varepsilon^{yy}$ of the main text, and derive the polarization dependences directly from these equations. We also discuss the key problems that one faces when describing the observed dynamics using a Néel vector $\mathbf{L}$.

## I. EXCITATION AND DETECTION OF COHERENT SPIN DYNAMICS AT TWO-MAGNON FREQUENCY IN TERMS OF THE SPIN CORRELATIONS

### A. Equation of motion of the spin correlations function

We consider the antiferromagnetic Heisenberg model,

$$\hat{H}_0 = J \sum_{i\boldsymbol{\delta}} \hat{\mathbf{S}}(\mathbf{r}_i)\hat{\mathbf{S}}(\mathbf{r}_i + \boldsymbol{\delta}) \tag{1}$$

where $i$ denotes lattice sites for magnetic ions at positions $\mathbf{r}_i$ and the index $\delta$ denotes nearest neighbor vectors $\boldsymbol{\delta} = (\delta^x, \delta^y, \delta^z)$. For the light-matter interaction, we consider laser-induced perturbation of exchange interactions. For cubic Mott insulators, only exchange bonds with a projection along the electric field are perturbed, as detailed in Ref. [1]. This allows us to write a phenomenological expression [1; 2] for the perturbation in the Hamiltonian by the electric field of the pump pulse.

$$\Delta\hat{H} = A(\omega) \sum_i \left[ \sum_{\boldsymbol{\delta}^x} \left(E^x \delta^x\right)^2 \hat{\mathbf{S}}(\mathbf{r}_i)\hat{\mathbf{S}}(\mathbf{r}_i + \boldsymbol{\delta}^x) + \sum_{\boldsymbol{\delta}^y} \left(E^y \delta^y\right)^2 \hat{\mathbf{S}}(\mathbf{r}_i)\hat{\mathbf{S}}(\mathbf{r}_i + \boldsymbol{\delta}^y) + \sum_{\boldsymbol{\delta}^z} \left(E^z \delta^z\right)^2 \hat{\mathbf{S}}(\mathbf{r}_i)\hat{\mathbf{S}}(\mathbf{r}_i + \boldsymbol{\delta}^z) \right], \tag{2}$$

where $\boldsymbol{\delta}^\nu$ is the vector in the direction of the $\nu$-axis of the crystal, $\nu = x, y, z$, e.g. $\boldsymbol{\delta}^x = (\delta^x, 0, 0)$ in Cartesian coordinates. $A(\omega)$ is a constant proportional to the strength of the perturbation of exchange interaction at the optical frequency $\omega$ and $E^\nu$ denotes the electric field of the laser pulse along the $\nu$-axis. Eq. (2) represents the bond-dependent part of the Hamiltonian for spontaneous Raman scattering from two-magnon modes presented in [2]. This is consistent with the physical picture that perturbations of exchange coupling along crystal bonds are responsible for the excitation of two-magnon modes. Indeed, the bond-independent part of the Raman tensor commutes with $\hat{H}_0$ and will not excite any spin dynamics.

We observe that the static and perturbed Hamiltonian are both translation invariant and related to spin correlations. The latter are evidently rotationally symmetric in spin space and hence independent of the orientation of the Neel vector. Therefore, we propose to develop a theory directly in terms of the dynamics of spin correlations, averaged over the total system:

$$\hat{C}(\boldsymbol{\delta}^\nu) = \sum_{i,\boldsymbol{\delta}^\nu} \hat{\mathbf{S}}(\mathbf{r}_i)\hat{\mathbf{S}}(\mathbf{r}_i + \boldsymbol{\delta}^\nu) = 2\sum_i \hat{\mathbf{S}}(\mathbf{r}_i)\hat{\mathbf{S}}(\mathbf{r}_i + \boldsymbol{\delta}^\nu), \tag{3}$$

* aleksei.kimel@ru.nl

where expectation value of $\hat{C}(\boldsymbol{\delta}^\nu)$ gives the spin correlations $\langle \hat{S}(\mathbf{r}_i)\hat{S}(\mathbf{r}_i+\boldsymbol{\delta},t)\rangle$, and the last equality holds for cubic crystals. The time-dependence of the operators is given in the Heisenberg representation. We note that the spin correlations of interest are distinctly different from those for incoherent one-magnon modes $\langle \hat{S}(\mathbf{r}_i,t)\hat{S}(\mathbf{r}_i,t')\rangle$ measured in experiments with neutron scattering. The incoherent counterpart of the two-magnon mode considered in our work can be studied using Raman scattering in the optical range and with Resonant Inelastic X-tay Scattering. In this case, the relevant spin correlation is $\langle \hat{S}(\mathbf{r}_i,t)\hat{S}(\mathbf{r}_i+\boldsymbol{\delta},t)\hat{S}(\mathbf{r}_i,t')\hat{S}(\mathbf{r}_i+\boldsymbol{\delta},t')\rangle$, which is a correlation in time between spin correlators, composed each of two spins separated by a bond $\boldsymbol{\delta}$.

In this notation, the total Hamiltonian of the system can be written as

$$\begin{aligned}\hat{H} = \hat{H}_0 + \Delta\hat{H} = \left[J + A(\omega)\left(E^x\delta^x\right)^2\right]\hat{C}(\boldsymbol{\delta}^x) \\ + \left[J + A(\omega)\left(E^y\delta^y\right)^2\right]\hat{C}(\boldsymbol{\delta}^y) + \left[J + A(\omega)\left(E^z\delta^z\right)^2\right]\hat{C}(\boldsymbol{\delta}^z)\end{aligned} \tag{4}$$

To derive the dynamics of spin correlations, we consider small transverse spin-deflections with respect to a collinear ground state. Keeping only the leading order contributions, we can identify three independent terms

$$\hat{C}_i^{(1)}(\boldsymbol{\delta}) = \frac{1}{2S}\left[\hat{S}^X(\mathbf{r}_i)\hat{S}^X(\mathbf{r}_i+\boldsymbol{\delta}) + \hat{S}^Y(\mathbf{r}_i)\hat{S}^Y(\mathbf{r}_i+\boldsymbol{\delta})\right], \tag{5}$$

$$\hat{C}_i^{(2)}(\boldsymbol{\delta}) = \frac{1}{2S}\left[\hat{S}^X(\mathbf{r}_i)\hat{S}^Y(\mathbf{r}_i+\boldsymbol{\delta}) - \hat{S}^Y(\mathbf{r}_i)\hat{S}^X(\mathbf{r}_i+\boldsymbol{\delta})\right], \tag{6}$$

$$\hat{C}_i^{(3)}(\boldsymbol{\delta}) = \frac{1}{4S}\left\{\left[\hat{S}^X(\mathbf{r}_i)\right]^2 + \left[\hat{S}^Y(\mathbf{r}_i)\right]^2 + \left[\hat{S}^X(\mathbf{r}_i+\boldsymbol{\delta})\right]^2 + \left[\hat{S}^Y(\mathbf{r}_i+\boldsymbol{\delta})\right]^2\right\}, \tag{7}$$

where $Z$ is the quantization axis. Note that in equilibrium, $\langle \hat{C}_i^{(2)}(\boldsymbol{\delta})\rangle = 0$, but it can be non-zero during dynamics. The total correlation can be written as

$$\sum_{\boldsymbol{\delta}^\nu}\hat{C}_i(\boldsymbol{\delta}^\nu) = 2\times 2S\left[\hat{C}_i^{(3)}(\boldsymbol{\delta}^\nu) + \hat{C}_i^{(1)}(\boldsymbol{\delta}^\nu)\right], \tag{8}$$

where we factored out the factor $2S$, which simplifies the calculation of commutators below. The factor 2 arises from the summation over $\boldsymbol{\delta}^\nu$. Constant terms $\sim -S^2$ were ignored since they do not contribute to the dynamics.

We note that spin correlations for different bonds are not independent: $[\hat{C}_i(\delta^\nu), \hat{C}_j(\delta^\mu)] \neq \delta_{ij}\delta_{\nu\mu}$, where $\delta_{ij}$ denotes the Kronecker delta, since they can share the same spin operator, for example, $\hat{\mathbf{S}}(\mathbf{r}_i+\boldsymbol{\delta}^\nu) = \hat{\mathbf{S}}(\mathbf{r}_j+\boldsymbol{\delta}^\mu)$. Physically, this means that, for example, the perturbation of exchange bonds along $x$ also triggers dynamics of spin correlations along $y$ and $z$. Therefore, it is more convenient to work in reciprocal space, which is achieved by the transformation

$$\hat{S}^X(\mathbf{r}_i) \pm i\hat{S}^Y(\mathbf{r}_i) = \sqrt{\frac{2}{N}}\sum_{\mathbf{k}}\hat{S}^{\pm}_{\mathbf{k}}e^{\pm i\mathbf{k}\mathbf{r}_i} \tag{9}$$

$$\hat{S}^X(\mathbf{r}_i+\boldsymbol{\delta}) \pm i\hat{S}^Y(\mathbf{r}_i+\boldsymbol{\delta}) = \sqrt{\frac{2}{N}}\sum_{\mathbf{k}}\hat{S}^{\pm}_{\mathbf{k}}e^{\mp i\mathbf{k}(\mathbf{r}_i+\boldsymbol{\delta})} \tag{10}$$

and the correlations can be written as

$$\begin{aligned}\hat{C}^{(1)}_{\mathbf{k}} &= \frac{1}{2S}\left(\hat{S}^X_{\mathbf{k}}\hat{S}^X_{-\mathbf{k}} + \hat{S}^Y_{\mathbf{k}}\hat{S}^Y_{-\mathbf{k}}\right), \\ \hat{C}^{(2)}_{\mathbf{k}} &= \frac{1}{2S}\left(\hat{S}^X_{\mathbf{k}}\hat{S}^Y_{-\mathbf{k}} - \hat{S}^Y_{\mathbf{k}}\hat{S}^X_{-\mathbf{k}}\right), \\ \hat{C}^{(3)}_{\mathbf{k}} &= \frac{1}{4S}\left[\left(\hat{S}^X_{\mathbf{k}}\right)^2 + \left(\hat{S}^Y_{\mathbf{k}}\right)^2 + \left(\hat{S}^X_{-\mathbf{k}}\right)^2 + \left(\hat{S}^Y_{-\mathbf{k}}\right)^2\right].\end{aligned} \tag{11}$$

and

$$\hat{C}_{\mathbf{k}}(\boldsymbol{\delta}^\nu) = 4S\left[\hat{C}^{(3)}_{\mathbf{k}} + \cos(\mathbf{k}\boldsymbol{\delta}^\nu)\hat{C}^{(1)}_{\mathbf{k}}\right], \tag{12}$$

where again the summation over $\boldsymbol{\delta}^\nu$ was taken. As follows directly from the commutations relations for the spin operators, the vector $\hat{\mathbf{C}}_{\mathbf{k}} = \left(\hat{C}^{(1)}_{\mathbf{k}}, \hat{C}^{(2)}_{\mathbf{k}}, \hat{C}^{(3)}_{\mathbf{k}}\right)$ satisfies the cross product in hyperbolic space: $\hat{\mathbf{C}}_{\mathbf{k}} \times \hat{\mathbf{C}}_{\mathbf{k}} = i\hbar\hat{\mathbf{C}}_{\mathbf{k}}$,

featuring a minus sign for the terms in the $\hat{C}^{(3)}_{\mathbf{k}}$ component as compared to the ordinary cross product. Hence, from Heisenberg equations of motion the dynamics of the correlations in reciprocal space are determined by

$$\hbar \frac{\partial \hat{\mathbf{C}}_{\mathbf{k}}}{\partial t} = \hat{\mathbf{C}}_{\mathbf{k}} \times \left( -\frac{\partial \hat{H}_{\mathbf{k}}}{\partial \hat{\mathbf{C}}_{\mathbf{k}}} \right) , \tag{13}$$

where the partial derivative also has an additional minus sign for the 3$^{\mathrm{rd}}$ component and the Hamiltonian in reciprocal space reads

$$\begin{aligned} \hat{H}_{\mathbf{k}} = J &\left[ \hat{C}_{\mathbf{k}}(\boldsymbol{\delta}^x) + \hat{C}_{\mathbf{k}}(\boldsymbol{\delta}^y) + \hat{C}_{\mathbf{k}}(\boldsymbol{\delta}^z) \right] \\ &+ A(\omega) E^2 \delta^2 \left[ \cos^2(\alpha) \hat{C}_{\mathbf{k}}(\boldsymbol{\delta}^x) + \sin^2(\alpha) \hat{C}_{\mathbf{k}}(\boldsymbol{\delta}^y) \right] , \end{aligned} \tag{14}$$

where $\tan(\alpha) = E^y/E^x$, $E^z = 0$, $E^2 = |\mathbf{E}|^2$ and $\delta^2 = |\boldsymbol{\delta}|^2$. Solving the equation of motion for impulsive perturbations yields oscillations of spin correlations dominated by the frequencies $\approx 2zJS/\hbar$, with $z = 6$ being the number of nearest neighbors [3], as discussed below.

### B. Modulation of the dielectric permittivity by the spin correlations dynamics and the polarization dependences

Next we show that the equation of motion for spin correlations indeed yields the polarization dependence on the pump pulse, as derived from phenomenological considerations in the main text. First, we note that from the light-matter interaction [Eq. (2)] it follows that the pump-induced dynamics of spin correlations contributes to the dielectric permittivity as

$$\Delta \varepsilon^{\nu\nu}(\omega_{pr}, \Delta t) = \eta^{\nu\nu}(\omega_{pr}) \sum_{\mathbf{k}} \Delta \left\langle \hat{C}_{\mathbf{k}}(\boldsymbol{\delta}^{\nu}, \Delta t) \right\rangle , \tag{15}$$

This equation accounts for the fact that the dynamics of spin corrections give rise only to the diagonal components of the dielectric tensor, since each magnetic ion in the cubic system has nearest neighbours only along the cubic axes. Note that dynamics of the spin correlation function can also be studied using other optical techniques. For example, magnetic linear dichroism is sensitive to $\hat{C}^{(3)}_{\mathbf{k}}$. The latter includes magnetic linear dichroism in the THz, optical, XUV, and X-ray spectral ranges.

Just as for ordinary Landau-Lifshitz equations, the pump-polarization dependence on $\hat{\mathbf{C}}_{\mathbf{k}}$ should follow from the pump-induced perturbation to the effective field $\mathbf{B}^{tot}_{\mathbf{k}} = -\partial \hat{H}_{\mathbf{k}} / \partial \hat{\mathbf{C}}_{\mathbf{k}}$. This can be decomposed as $\mathbf{B}^{\mathrm{tot}}_{\mathbf{k}} = \mathbf{B}_{\mathbf{k}} + \Delta \mathbf{B}_{\mathbf{k}}$. The individual components read $B^{(2)}_{\mathbf{k}} = 0 = \Delta B^{(2)}_{\mathbf{k}}$, $B^{(3)}_{\mathbf{k}} = 2zJS$, $\Delta B^{(3)}_{\mathbf{k}} = 4SA(\omega_p)E^2\delta^2$, and for the 1$^{\mathrm{st}}$-components we get

$$B^{(1)}_{\mathbf{k}} = -\frac{B^{(3)}_{\mathbf{k}}}{3} \left[ \cos(\mathbf{k}\boldsymbol{\delta}^x) + \cos(\mathbf{k}\boldsymbol{\delta}^y) + \cos(\mathbf{k}\boldsymbol{\delta}^z) \right] , \tag{16}$$

$$\begin{aligned} \Delta B^{(1)}_{\mathbf{k}} &= -\frac{\Delta B^{(3)}_{\mathbf{k}}}{2} \cos(2\alpha) \left[ \cos(\mathbf{k}\boldsymbol{\delta}^x) - \cos(\mathbf{k}\boldsymbol{\delta}^y) \right] \\ &\quad - \frac{\Delta B^{(3)}_{\mathbf{k}}}{2} \left[ \cos(\mathbf{k}\boldsymbol{\delta}^x) + \cos(\mathbf{k}\boldsymbol{\delta}^y) \right] . \end{aligned} \tag{17}$$

The amplitude of the induced oscillations are proportional to $|\Delta \mathbf{B}^{\perp}_{\mathbf{k}}|$, where

$$\begin{aligned} \Delta \mathbf{B}^{\perp}_{\mathbf{k}} &= \frac{1}{|\mathbf{B}_{\mathbf{k}}|^2} \mathbf{B}_{\mathbf{k}} \times (\mathbf{B}_{\mathbf{k}} \times \Delta \mathbf{B}_{\mathbf{k}}) \\ &= \frac{1}{|\mathbf{B}_{\mathbf{k}}|^2} \left( B^{(3)}_{\mathbf{k}} B^{(1)}_{\mathbf{k}} \Delta B^{(3)}_{\mathbf{k}} - B^{(3)}_{\mathbf{k}} B^{(3)}_{\mathbf{k}} \Delta B^{(1)}_{\mathbf{k}}, 0, B^{(1)}_{\mathbf{k}} B^{(1)}_{\mathbf{k}} \Delta B^{(3)}_{\mathbf{k}} - B^{(1)}_{\mathbf{k}} B^{(3)}_{\mathbf{k}} \Delta B^{(1)}_{\mathbf{k}} \right) \\ &= \frac{B^{(1)}_{\mathbf{k}} \Delta B^{(3)}_{\mathbf{k}} - B^{(3)}_{\mathbf{k}} \Delta B^{(1)}_{\mathbf{k}}}{|\mathbf{B}_{\mathbf{k}}|^2} \left( B^{(3)}_{\mathbf{k}}, 0, B^{(1)}_{\mathbf{k}} \right) . \end{aligned} \tag{18}$$

Having defined effective field and its deviation responsible for the excitation of the dynamics of $\hat{\mathbf{C}}_{\mathbf{k}}$, we can now write down a solution of the equation of motion [Eq. (13)] in analogy to the Landau-Lifshitz equation for magnetization as

$$\Delta\langle \hat{C}^{(1)}_{\mathbf{k}}\rangle \propto |\Delta \mathbf{B}^{\perp}_{\mathbf{k}}| \sin\left(\frac{|\mathbf{B}_{\mathbf{k}}|}{\hbar}\Delta t\right). \tag{19}$$

Then, using Eq. (15) we obtain an expression which relates laser-induced change of the effective field and induced optical birefringence:

$$\begin{aligned}
\varepsilon^{xx} - \varepsilon^{yy} &\propto \sum_{\mathbf{k}} \Delta\langle \hat{C}^{(1)}_{\mathbf{k}}\rangle \left[\cos(\mathbf{k}\boldsymbol{\delta}^x) - \cos(\mathbf{k}\boldsymbol{\delta}^y)\right] \\
&\propto \sum_{\mathbf{k}} |\Delta \mathbf{B}^{\perp}_{\mathbf{k}}| \left[\cos(\mathbf{k}\boldsymbol{\delta}^x) - \cos(\mathbf{k}\boldsymbol{\delta}^y)\right] \\
&= \sum_{\mathbf{k}} \frac{\Delta B^{(3)}_{\mathbf{k}}}{6|\mathbf{B}_{\mathbf{k}}|} \left\{3\cos(2\alpha)\left[\cos(\mathbf{k}\boldsymbol{\delta}^x) - \cos(\mathbf{k}\boldsymbol{\delta}^y)\right]\right. \\
&\qquad \left. + \cos(\mathbf{k}\boldsymbol{\delta}^x) + \cos(\mathbf{k}\boldsymbol{\delta}^y) - 2\cos(\mathbf{k}\boldsymbol{\delta}^z)\right\} \left[\cos(\mathbf{k}\boldsymbol{\delta}^x) - \cos(\mathbf{k}\boldsymbol{\delta}^y)\right] \\
&= \sum_{\mathbf{k}} \frac{\Delta B^{(3)}_{\mathbf{k}}}{2|\mathbf{B}_{\mathbf{k}}|} \cos(2\alpha) \left[\cos(\mathbf{k}\boldsymbol{\delta}^x) - \cos(\mathbf{k}\boldsymbol{\delta}^y)\right]^2 \\
&\quad + \sum_{\mathbf{k}} \frac{\Delta B^{(3)}_{\mathbf{k}}}{6|\mathbf{B}_{\mathbf{k}}|} \left[\cos(\mathbf{k}\boldsymbol{\delta}^x) + \cos(\mathbf{k}\boldsymbol{\delta}^y) - 2\cos(\mathbf{k}\boldsymbol{\delta}^z)\right] \left[\cos(\mathbf{k}\boldsymbol{\delta}^x) - \cos(\mathbf{k}\boldsymbol{\delta}^y)\right].
\end{aligned} \tag{20}$$

Here, for a sake of simplicity we omitted the time-dependent part and focused on the amplitude of modulation only. The second term vanishes under summation over the whole Brillouin zone, since $\Delta B^{(3)}_{\mathbf{k}}$ is independent of $\mathbf{k}$, and $|\mathbf{B}_{\mathbf{k}}|$ is even in $\mathbf{k}$. The final expression for the transient optical birefrigence takes the form:

$$(\varepsilon^{xx} - \varepsilon^{yy})(\Delta t) \propto \cos(2\alpha) \sum_{\mathbf{k}} \frac{\left[\cos(\mathbf{k}\boldsymbol{\delta}^x) - \cos(\mathbf{k}\boldsymbol{\delta}^y)\right]^2}{2|\mathbf{B}_{\mathbf{k}}|} \sin\left(\frac{|\mathbf{B}_{\mathbf{k}}|}{\hbar}\Delta t\right) \tag{21}$$

Hence, we recover the $\cos(2\alpha)$ dependence of the laser-induced dynamics of optical birefringence directly from the equations of motion for spin correlations, in accordance with the symmetry analysis in the main text. Oscillations of optical birefringence are dominated by the two-magnon mode frequency $\approx 2zJS/\hbar$.

Finally, using standard Jones matrix formalism, we obtain an expression for the amplitude of the modulation of the probe ellipticity dependent on the incident probe polarization $\beta$:

$$\Delta\beta = \frac{\omega d\left[\varepsilon^{xx} - \varepsilon^{yy}\right]}{4c\sqrt{\varepsilon^{xx}}} \sin(2\beta) \propto \cos(2\alpha)\sin(2\beta), \tag{22}$$

that fully describes the experimentally observed polarization dependences [Fig. 3(d) in the main text].

Using the expressions derived above, we calculated the transient ellipticity $\Delta\beta(t)$ [Fig. 3(c) in the main text]. In the calculations, the following parameters of $RbMnF_3$ were used: $J = 0.52$ meV, $S = 5/2$, $z = 6$ [4], duration of the pump pulse $\tau_p = 45$ fs. The laser-induced perturbation of the exchange coupling was of $-1$ % shown earlier to be a realistic value [3]. In the calculations, the incident probe polarization angle was $\beta = 45, 135°$, and the pump polarization angle was $\alpha = 0,\ 90°$. We note that our model does not account for the magnon-magnon interactions, which shift the maximum of spectral amplitude from the highest frequency to the lower frequencies. Therefore, $J$ used in the calculations is at the lower limit of the range of values reported in the literature [4]. The calculations yield oscillations of the probe ellipticity at the dominating frequency of 4 THz, which is in good agreement with the experimental result. Oscillations induced by pump pulses with orthogonal polarizations possess opposite initial phase, as also seen in experiments [compare Figs. 3(a,c) in the main text]. The rotation of the incident probe polarization from $\beta = 45°$ to $135°$ resulted in the phase change by $\pi$ in agreement with experiments [Fig. 3(b) in the main text].

## II. DESCRIPTION OF COHERENT SPIN DYNAMICS AT TWO-MAGNON FREQUENCY IN TERMS OF THE MACROSPIN APPROXIMATION

### A. Dynamics of magnetic linear birefringence

We start from examining an assumption that the observed modulation of the probe ellipticity could stem from transient magnetic linear birefringence (MLB) and thus is linked to the dynamics of $\mathbf{L}$, either transverse or longitudinal.

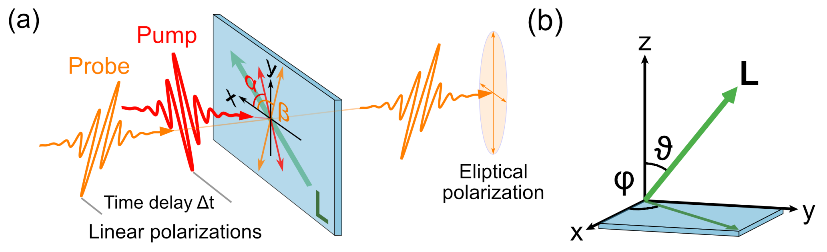


FIG. S1. (a) Schematic of the experimental geometry. Linearly polarized ultrashort optical pump pulse excites ultrafast spin dynamics which is detected via induced ellipticity changes of the time delayed optical probe pulse. (b) The antiferromagnetic vector **L** and its projection on the $xy$ plane in the sample of $RbMnF_3$.

For the point group $m\bar{3}m$ of $RbMnF_3$ one find that magneto-optical susceptibility $\zeta^{ijkl}$ describing MLB ($\varepsilon^{ij} = \zeta^{ijkl}L^kL^l$) has only two independent components, $\zeta^{iiii} = a$ and $\zeta^{iijj} = \zeta^{ijij} = \zeta^{ijji} = b$, where $i, j, k, l = x, y, z$ [5]. The dielectric permittivity tensor components relevant for the probe pulses propagating along $z$ axis are:

$$\begin{aligned} \varepsilon^{xx} &= \varepsilon^0 + a(L^x)^2 + b[(L^y)^2 + (L^z)^2]; \\ \varepsilon^{yy} &= \varepsilon^0 + a(L^y)^2 + b[(L^x)^2 + (L^z)^2]; \\ \varepsilon^{xy} &= \varepsilon^{yx} = 2bL^xL^y, \end{aligned} \tag{23}$$

where $\varepsilon^0$ stands the diagonal components of the dielectric permittivity tensor without magnetic ordering. Using definition of the angles $\phi$ and $\theta$ [Fig. S1(b)] the components **L** are $L^x = L_0 \cos\phi \sin\theta$, $L^y = L_0 \sin\phi \sin\theta$, and $L^z = L_0 \cos\theta$, with $L_0$ being the length of **L**.

In the static case with $\mathbf{L}\|[111]$ ($\phi = 45°$; $\theta = 54.74°$) one finds that the eigen polarizations are the two waves propagating along the $z$ axis and linearly polarized at angles 45° with respect to the $x$ and $y$ axes. The difference in the refraction indices for these two waves is

$$\Delta n = n_1 - n_2 = \frac{4bL_0^2}{3\sqrt{\varepsilon^0}}, \tag{24}$$

where we used a reasonable assumption that magnetic contribution to the dielectric permittivity is weaker than the nonmagnetic one, $a(L^i)^2; b(L^i)^2 << \varepsilon^0$. In the basis formed by the two eigen polarizations, the electric field of the probe pulse polarized at an angle $\beta$ [Fig. S1(a)] has the components $E_1 = E_0 \cos(\phi - \beta)$, $E_2 = E_0 \sin(\phi - \beta)$. Then such pulse pulse acquires ellipticity after traversing the sample of thickness $d$:

$$\Delta\beta = \frac{\omega d[n_1^2 - n_2^2]}{4c\sqrt{\varepsilon^0}} \sin(2(\phi - \beta)) = \frac{\omega d}{3c\sqrt{\varepsilon^0}} bL_0^2 \sin(2(\phi - \beta)), \tag{25}$$

which gives the $\cos(2\beta)$ dependence at $\phi = 45°$, as expected for the MLB being the largest when the light polarization makes an angle 45° with the main axes, given by the projection of **L** on $xy$ plane.

We now assume, following [6; 7], that the perturbation of the exchange coupling results in *longitudinal* oscillations of the length of the antiferromagnetic vector $|\mathbf{L}(t)| = L_0 + l_0 \sin(2\Omega_{\pi/a}t)$. The amplitude of the oscillations $l_0$ scales linearly with the laser fluence, as the off-resonant optical excitation of spin dynamics is the down-conversion process involving two photons. In experiments the amplitude of the transient ellipticity scales linearly with pump fluence as well, and we can limit our consideration to the terms linear in $l_0$. Then from Eq. (25) one gets the expression for the time-dependent ellipticity of the probe pulse:

$$\Delta\beta(t) = \frac{2\omega d}{3c\sqrt{\varepsilon^0}} bL_0 \sin(2(\phi - \beta)) l_0 \sin(2\Omega_{\pi/a}t). \tag{26}$$

As can be seen, at $\phi = 45°$, the expected probe polarization dependence $\cos(2\beta)$ clearly different from $\sin(2\beta)$-dependence found in experiments [Fig. 3(c) in the main text].

Next we assume *transverse* oscillation of **L** that can be described by introducing deviations of the angles $\phi + \delta\phi(t)$ and $\theta + \delta\theta(t)$. Dynamical changes of $\theta + \delta\theta(t)$ affect projection of **L** on the $xy$ plane. In the considered geometry it is similar to oscillations of its length $l_0$, and thus, such dynamics does not yield the correct probe polarization dependence. The emergence of $\delta\phi(t)$ would result in the modulation of the probe ellipticity following the dependence $\sin(2(\phi - \beta) + 2\delta\phi(t))$. Limiting consideration to terms linear in small deviations $\delta\phi(t)$ one gets

$$\Delta\beta(t) = \frac{2\omega d}{3c\sqrt{\varepsilon^0}} bL_0^2 \cos(2(\phi - \beta))\delta\phi(t). \tag{27}$$

At $\phi = 45°$ the transient ellipticity related to the transversal oscillations of $\mathbf{L}$ do follow $\sin 2\beta$-dependence observed in experiments. However, such assumption leads to the paradoxical conclusion that the antiferromagnetic vector can precess at the frequency $2\Omega_{\pi/a}$ and this precession should be quasi-homogeneous in order to be probed optically.

### B. Concomitant detection of two spin waves via MLB

Homogeneous modulation of $\phi$ at the doubled spin waves frequency $\Omega_k$ may only stem from concomitant detection of two spin waves with opposite wavevectors. Indeed, within a macrospin approcah a spin wave can be described by introducing inhomogeneous modulation of the angles describing orientation of $\mathbf{L}$:

$$\phi(\Omega_k, \mathbf{k}) = \delta\phi_{0;\mathbf{k}} e^{-i\mathbf{kr}} e^{-i\Omega_{\mathbf{k}} t}. \tag{28}$$

where $\delta\phi_{0;\mathbf{k}}$ is the spin wave amplitude and $\Omega_k \leq \Omega_{\pi/a}$. In the case of off-resonant excitation, the spin-wave amplitude can be only linear in laser fluence. However, detection of the homogeneous modulation of MLB at the frequency $2\Omega_k$ requires detection of the pair of the waves such as $\Delta\beta(t) \propto \phi(\Omega_k, \mathbf{k}) \cdot \phi(\Omega_k, -\mathbf{k}) = (\delta\phi_{0;k})^2 \sin(2\Omega_k t)$. The amplitude of such modulation of the probe ellipticity is, however, quadratic in the pump fuence, and such scenario of the detection of the concominant spin waves can be ruled out.

### C. Inverse magnetic refraction

Limiting ourselves with exchange interactions only and neglecting spin-orbit interactions, we arrive to the following possible scenario of excitation of the two-magnon mode based on the macrospin approximation. Under such constrains, there is a term in the energy of light-matter interaction $U_{\mathrm{ex}} = \zeta^{ii}(E^i)^2(L_0)^2$, $i = x, y, z$, which describes the effect known as a magnetic refraction stemming from the exchange contribution to optical susceptibility of a medium [8]. In $RbMnF_3$, this effect is an isotropic change of the refractive index in the magnetically-ordered phase. Here $\zeta^{ii}$ is written for the $m\bar{3}m$ point group [5], and $(L_0)^2$ accounts for the fact that the effect is present in the magnetically-ordered phase and is independent from the orientation on $\mathbf{L}$.

The presence of such contribution means that light can perturb exchange coupling. However, since this term is isotropic with respect to both the electric field of light ($\zeta^{xx} = \zeta^{yy} = \zeta^{zz}$ [5]) and the antiferromagnetic vector, it would yield that the excitation of the related spin dynamics is isotropic with respect to the polarization of the exciting pulse. This, clearly, contradicts the experimental observations in this work and in Ref. [6].


[1] J. Mentink, K. Balzer, and M. Eckstein, Ultrafast and reversible control of the exchange interaction in Mott insulators, Nat. Commun. **6**, 6708 (2015).

[2] R. J. Elliott and M. F. Thorpe, The effects of magnon-magnon interaction on the two-magnon spectra of antiferromagnets, J. Phys. C: Solid State Phys. **2**, 1630 (1969).

[3] A. E. Fedianin, A. M. Kalashnikova, and J. H. Mentink, Selection rules for ultrafast laser excitation and detection of spin correlation dynamics in a cubic antiferromagnet, Phys. Rev. B **107**, 144430 (2023).

[4] C. G. Windsor and R. W. H. Stevenson, Spin waves in $RbMnF_3$, Proc. Phys. Soc. **87**, 501 (1966).

[5] R. R. Birss, Symmetry and magnetism (North-Holland Amsterdam, 1964).

[6] D. Bossini, S. Dal Conte, G. Cerullo, O. Gomonay, R. V. Pisarev, M. Borovsak, D. Mihailovic, J. Sinova, J. H. Mentink, T. Rasing, and A. V. Kimel, Laser-driven quantum magnonics and terahertz dynamics of the order parameter in antiferromagnets, Phys. Rev. B **100**, 024428 (2019).

[7] D. Bossini, S. Dal Conte, Y. Hashimoto, A. Secchi, R. V. Pisarev, T. Rasing, G. Cerullo, and A. V. Kimel, Macrospin dynamics in antiferromagnets triggered by sub-20 femtosecond injection of nanomagnons, Nat. Commun. **7**, 10645 (2016).

[8] B. B. Krichevtsov, P. A. Markovin, S. V. Petrov, and R. V. Pisarev, Isotropic and anisotropic magnetic refraction of light in the antiferromagnets $KNiF_3$ and $RbMnF_3$, Sov. Phys. JETP **59**, 1316 (1984).
